# Supplementary material for: Analyzing User Ideologies and Shared News During the 2019 Argentinian Elections
Source: arXiv:2310.08701 source file (2024-04-25)
Supplement: Supplementary file 1 [file SI.pdf]

# Biased news sharing and partisan polarization on social media
## Supplementary information

Sofía M del Pozo[12], Sebastián Pinto[12], Matteo Serafino[3], Lucio Garcia[12], Hernán A Makse[4] and Pablo Balenzuela[12].

[1] Universidad de Buenos Aires, Facultad de Ciencias Exactas y Naturales, Departamento de Física. Buenos Aires, Argentina.

[2] CONICET - Universidad de Buenos Aires, Instituto de Física Interdisciplinaria y Aplicada (INFINA). Buenos Aires, Argentina.

[3]IMT Institute for Advanced Studies, 55100 Lucca, Italy.

[4]Levich Institute and Physics Department, City College of New York, 10031 New York, USA.

October 12, 2023

## 1 News articles by partisans

Figure 1 shows the amount of news articles shared by users with Center-Left and Center-Right leanings for each media outlet. Media outlets in red were excluded from the $\bar{SB}$ analysis in Fig. 3 of the main text.

## 2 Topics of news articles

Figure 2 shows the wordclouds of the topics cited in the main text. Tables 1 and 2 shows examples of related articles for each topic.

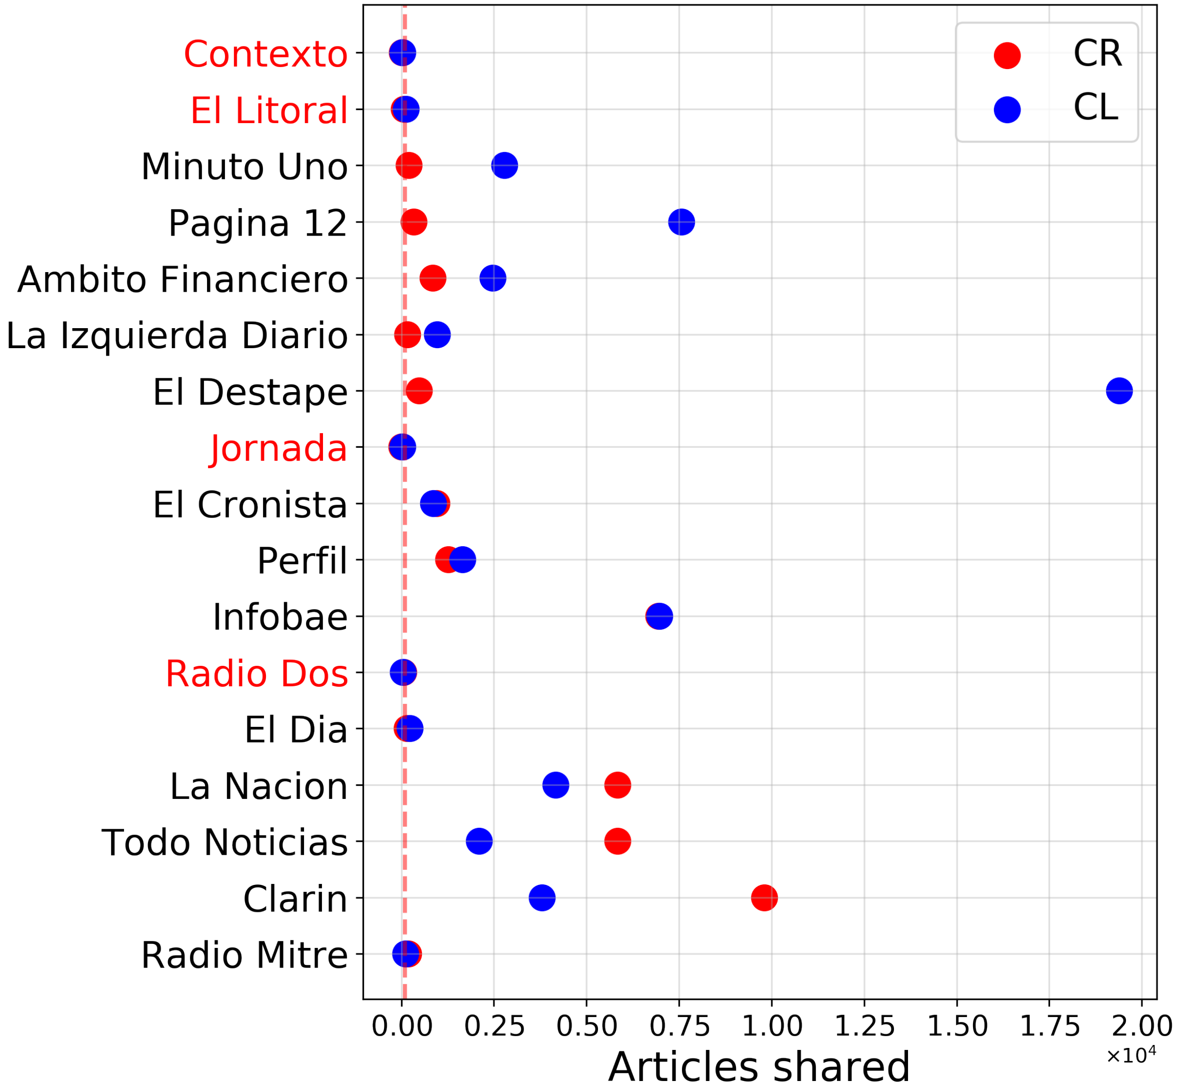


Figure 1: **Amount of news articles shared by users with Center-Left (blue) and Center-Right (red) leanings.** The red line represents the threshold of 100, which is when we began including media outlets for $\bar{SB}$ analysis in Fig. 3 in the main text. Media outlets in red have less than 100 news articles shared by at least one group of users.

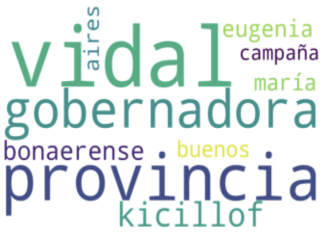


(a) Politics BA province.

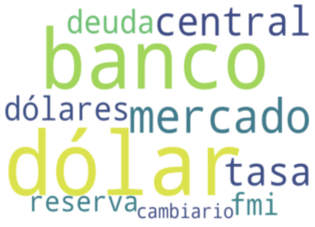


(b) Economy/Dolar.

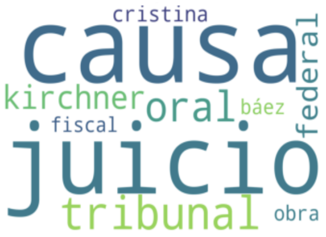


(c) Justice.

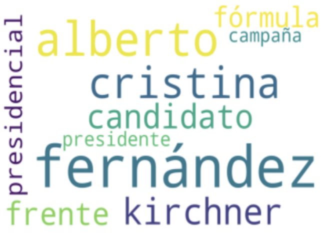


(d) Politics CL.

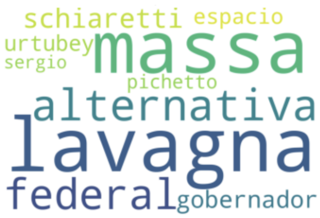


(e) 3rd Party.

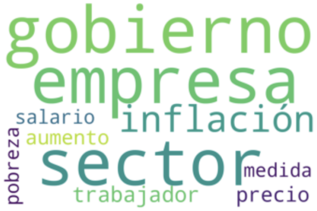


(f) Wage/Inflation.

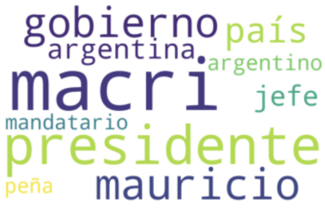


(g) Politics CR.

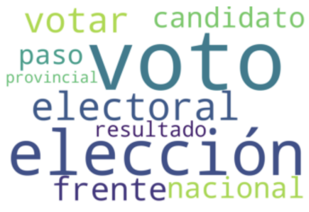


(h) Elections.

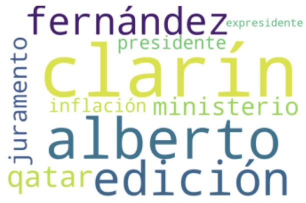


(i) Trash topic.

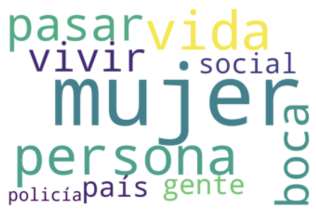


(j) Gossip & Sports.

Figure 2: Wordcloud of topics. Example articles are referred in each case.

| **Topics** | **Examples of News Articles** |
|---|---|
| Politics BA Province | El Destape: "Debate 2019: qué dijo María Eugenia Vidal tras el fallido de Macri en el que dio a Kicillof como gobernador" [1], Pagina 12: "Un café amargo para María Eugenia Vidal" [2], La Nacion: "Así es la cumbia de Vidal que busca captar el voto bonaerense" [3] |
| Economy/Dolar | La Nacion: "El dólar subió hoy 80 centavos por la pelea de Trump con China" [4], El Destape: "Dólar hoy: subió más de 30 centavos y cerró a $ 40,13" [5], Todo Noticias: "El Banco Central y las elecciones: dólar bajo control hasta las PASO y tasas altas por cinco meses" [6] |
| Justice | Infobae: "La Fiscalía solicitó unificar las causas 'Hotesur' y 'Los Sauces' y que Cristina Kirchner sea juzgada en un solo juicio oral" [7], La Nacion: "Cristina fue a Comodoro Py para notificarse de los nuevos procesamientos" [8], Todo Noticias: "Lázaro Báez pidió suspender el juicio que tiene a Cristina como principal acusada" [9] |
| Politics CL | La Nacion: "Los mejores memes por el anuncio de Cristina Kirchner como vicepresidenta de Alberto Fernández" [10], El Destape: "Alberto Fernández le contestó a Cambiemos: 'Cristina no es Perón y yo no soy Cámpora'" [11], Pagina 12: "Romano: 'La figura de Alberto Fernández es inspiradora'" [12] |
| 3rd Party | La Nacion: "Lifschitz y Stolbizer evitaron una ruptura definitiva de Lavagna con Alternativa Federal" [13], Todo Noticias: "Roberto Lavagna: 'No hubo ninguna ruptura con Alternativa Federal, todos los diálogos están abiertos'" [14], Pagina 12: "Tensión en el peronismo disidente por la estrategia electoral" [15] |
| Wage/Inflation | Clarin: "A marzo, los sueldos perdieron 10,5% de su poder adquisitivo" [16], Pagina 12: "Fuerte retroceso de la industria" [17], El Destape: "La eliminación del IVA beneficiará más a sectores de mayor ingreso que a los más pobres" [18] |
| Politics CR | Pagina 12: "Macri se compara con San Martín" [19], El Destape: "El insólito audio de Faurie a Macri contándole el acuerdo entre Mercosur – Unión Europea" [20], Clarin: "Mauricio Macri, en modo campaña en un acto por el 25 de Mayo: 'Volver atrás sería destruirnos'" [21] |

Table 1

| Topics | Examples of News Articles |
| --- | --- |
| Elections | Pagina 12: "Los datos crudos del escrutinio definitivo" [22], La Nacion: "Resultados de las Elecciones en Antártida Argentina: seguí el recuento de votos de las PASO" [23], Clarin: "Voto en blanco: no se contará en octubre y hay más chance de definir en primera vuelta" [24] |
| Trash topic | Clarin: ’"Esto no es sarasa": el video de Mauricio Macri en la celebración de los 10 años de los centros de Primera Infancia’ [25], Clarin: "Massa: ’Los voy a meter presos’" [26], Clarin: "La obra en el arroyo el Gato y el ’autohomenaje’ de Macri" [27] |
| Gossip & Sport | "El deseo de buena suerte de Alessandro Del Piero antes del debut de Daniele De Rossi" [28], ’"¿Quién es ese? No lo conozco, lo veré en el Monumental": el "Beto" Alonso menospreció a Daniele De Rossi’ [29], "De Rossi se dio el gusto: cómo vivió su primer partido con Boca en la Bombonera" [30] |

Table 2

# References


[1] *Debate 2019: qué dijo María Eugenia Vidal tras el fallido de Macri en el que dio a Kicillof como gobernador.* https://www.eldestapeweb.com/nota/debate-2019-que-dijo-maria-eugenia-vidal-tras-el-fallido-de-macri-en-el-que-dio-a-kicillof-como-gobernador-201910159140.

[2] *Un café amargo para María Eugenia Vidal.* https://www.pagina12.com.ar/216327-un-cafe-amargo-para-maria-eugenia-vidal.

[3] *Así es la cumbia de Vidal que busca captar el voto bonaerense.* https://www.lanacion.com.ar/politica/asi-es-cumbia-vidal-busca-captar-voto-nid2272995/.

[4] *El dólar subió hoy 80 centavos por la pelea de Trump con China.* https://www.lanacion.com.ar/economia/dolar/la-pelea-trump-china-le-pone-mas-nid2274338/.

[5] *Dólar hoy: subió más de 30 centavos y cerró a $ 40,13.* https://www.eldestapeweb.com/dolar-hoy-subio-mas-30-centavos-y-cerro-4013-n56710.

[6] *El Banco Central y las elecciones: dólar bajo control hasta las PASO y tasas altas por cinco meses.* https://tn.com.ar/economia/el-banco-central-y-las-elecciones-dolar-bajo-control-hasta-las-paso-y-tasas-altas-por-cinco-meses_980295/.

[7] *La Fiscalía solicitó unificar las causas "Hotesur" y "Los Sauces" y que Cristina Kirchner sea juzgada en un solo juicio oral.* https://www.infobae.com/politica/2019/03/28/la-fiscalia-solicito-unificar-las-causas-hotesur-y-los-sauces-y-que-cristina-kirchner-sea-juzgada-en-un-solo-juicio-oral/.

[8] *Cristina fue a Comodoro Py para notificarse de los nuevos procesamientos.* https://www.lanacion.com.ar/politica/cristina-fue-comodoro-py-notificarse-nuevos-procesamientos-nid2232956/.

[9] *Lázaro Báez pidió suspender el juicio que tiene a Cristina como principal acusada.* https://tn.com.ar/politica/lazaro-baez-pidio-suspender-el-primer-juicio-cristina-por-corrupcion_963358/.

[10] *Los mejores memes por el anuncio de Cristina Kirchner como vicepresidenta de Alberto Fernández.* https://www.lanacion.com.ar/politica/los-mejores-memes-anuncio-cristina-kirchner-como-nid2249212/.

[11] *Alberto Fernández le contestó a Cambiemos: "Cristina no es Perón y yo no soy Cámpora".* https://www.eldestapeweb.com/c60160.

[12] *Romano: "La figura de Alberto Fernández es inspiradora".* https://www.pagina12.com.ar/449426-romano-la-figura-de-alberto-fernandez-es-inspiradora.

[13] *Lifschitz y Stolbizer evitaron una ruptura definitiva de Lavagna con Alternativa Federal.* https://www.lanacion.com.ar/politica/lifschitz-stolbizer-evitaron-ruptura-definitiva-lavagna-alternativa-nid2250539/.

[14] *Roberto Lavagna: "No hubo ninguna ruptura con Alternativa Federal, todos los diálogos están abiertos".* https://tn.com.ar/politica/roberto-lavagna-no-hubo-una-ruptura-con-alternativa-federal-sino-diferencias_964627/.

[15] *Tensión en el peronismo disidente por la estrategia electoral.* https://www.pagina12.com.ar/195430-tension-en-el-peronismo-disidente-por-la-estrategia-electora.

[16] *A marzo, los sueldos perdieron 10,5% de su poder adquisitivo.* https://www.clarin.com/economia/economia/marzo-sueldos-perdieron-10-poder-adquisitivo_0_7Sa7fPyvR.html.

[17] *Fuerte retroceso de la industria.* https://www.pagina12.com.ar/204353-fuerte-retroceso-de-la-industria.

[18] *La eliminación del IVA beneficiará más a sectores de mayor ingreso que a los más pobres.* https://www.eldestapeweb.com/nota/la-eliminacion-del-iva-beneficiara-mas-a-sectores-de-mayor-ingreso-que-a-los-mas-pobres-201982617140.

[19] *Macri se compara con San Martín.* https://www.pagina12.com.ar/449941-macri-se-compara-con-san-martin.

[20] *El insólito audio de Faurie a Macri contándole el acuerdo entre Mercosur – Unión Europea.* https://www.eldestapeweb.com/nota/el-insolito-audio-de-faurie-a-macri-contandole-el-acuerdo-entre-mercosur-union-europea-20196281590.

[21] *Mauricio Macri, en modo campaña en un acto por el 25 de Mayo: "Volver atrás sería destruirnos".* https://www.clarin.com/politica/mauricio-macri-modo-campana-acto-25-mayo-volver-destruirnos_0_U975lZ07h.html.

[22] *Los datos crudos del escrutinio definitivo.* https://www.pagina12.com.ar/201768-los-datos-crudos-del-escrutinio-definitivo.

[23] *Resultados de las Elecciones en Antártida Argentina: seguí el recuento de votos de las PASO.* https://www.lanacion.com.ar/politica/resultados-de-las-elecciones-en-antartida-argentina-segui-el-recuento-de-votos-nid2280334/.

[24] *Voto en blanco: no se contará en octubre y hay más chance de definir en primera vuelta.* https://www.clarin.com/politica/voto-blanco-contara-octubre-chance-definir-primera-vuelta_0_WYzHzdszB.html.

[25] *"Esto no es sarasa": el video de Mauricio Macri en la celebración de los 10 años de los centros de Primera Infancia*. https://www.clarin.com/politica/sarasa-video-mauricio-macri-celebracion-10-anos-centros-primera-infancia_3_FuZVIgtG3.html.

[26] *Massa: "Los voy a meter presos"*. https://www.clarin.com/politica/massa-voy-meter-presos_3_S1xG3wPngz.html.

[27] *La obra en el arroyo el Gato y el "autohomenaje" de Macri*. https://www.clarin.com/videos/obra-arroyo-gato-autohomenaje-macri_3_1uyuSPoA4.html.

[28] *El deseo de buena suerte de Alessandro Del Piero antes del debut de Daniele De Rossi*. https://www.clarin.com/boca-juniors/deseo-buena-suerte-alessandro-piero-debut-daniele-rossi_0_g3kWd1TQQ.html.

[29] *"¿Quién es ese? No lo conozco, lo veré en el Monumental": el "Beto" Alonso menospreció a Daniele De Rossi*. https://www.infobae.com/deportes-2/2019/08/13/quien-es-ese-no-lo-conozco-lo-vere-en-el-monumental-el-beto-alonso-menosprecio-a-daniele-de-rossi/.

[30] *De Rossi se dio el gusto: cómo vivió su primer partido con Boca en la Bombonera*. https://www.lanacion.com.ar/deportes/futbol/de-rossi-se-dio-gusto-como-vivio-nid2278767/.
